# Supplementary material for: A dispersive study of final-state interactions in $K\to\pi\pi\pi$ amplitudes
Source: arXiv:2403.17570 ancillary file (2024-03-26)
Supplement: Supplementary file 1 [file KT_Pto3pi_README.pdf]

# README file for the ancillary files to A dispersive study of final-state interactions in $K \rightarrow \pi\pi\pi$ amplitudes

Véronique Bernard<sup>1\*</sup>, Sébastien Descotes-Genon<sup>1†</sup>, Marc Knecht<sup>2‡</sup>, Bachir Moussallam<sup>1§</sup>

<sup>1</sup>*Université Paris-Saclay, CNRS/IN2P3, IJCLab, 91405 Orsay, France*

<sup>2</sup>*Centre de Physique Théorique, CNRS/Aix-Marseille Univ./Univ. de Toulon (UMR7332)  
CNRS-Luminy Case 907, 13288 Marseille Cedex 9, France*

The present text provides a description of the content of the ancillary files to the solution of the Omnès-Khuri-Treiman-Sawyer-Wali integral equations for the  $K \rightarrow \pi\pi\pi$  amplitudes. These solutions are expressed as linear combinations of a set of fundamental functions ( $I$  is an isospin label)

$$\begin{aligned} \begin{pmatrix} M_I(s) \\ N_I(s) \end{pmatrix} &= \begin{pmatrix} \mu_0 \\ \nu_0 \end{pmatrix} \mathcal{S}_I^{(0)}(s) + \begin{pmatrix} \mu_1 \\ \nu_1 \end{pmatrix} \mathcal{S}_I^{(1)}(s) + \begin{pmatrix} \mu_2 \\ \nu_2 \end{pmatrix} \mathcal{S}_I^{(2)}(s) + \begin{pmatrix} \mu_3 \\ \nu_3 \end{pmatrix} \mathcal{S}_I^{(3)}(s), \quad I = 0, 1, 2 \\ \tilde{M}_1(s) &= \tilde{\mu}_1 \tilde{\mathcal{S}}_1(s), \quad \tilde{N}_1(s) = \tilde{\nu}_0 \tilde{\mathcal{S}}_1^{(0)} + \tilde{\nu}_1 \tilde{\mathcal{S}}_1^{(1)}, \quad I = 1, 2, \end{aligned} \tag{1}$$

modulated by the complex coefficients  $\mu_n, \nu_n, \tilde{\nu}_{0,1}, \tilde{\mu}_1$ . Some of these coefficients and fundamental functions carry dimensions, and will be given in units of  $\text{GeV}^N$ , with  $N$  as given in the following Table:

| $N$ | coefficients                                               | fundamental functions                                                                                                                                                 |
|-----|------------------------------------------------------------|-----------------------------------------------------------------------------------------------------------------------------------------------------------------------|
| −4  | $\mu_2, \mu_3, \nu_2, \nu_3, \tilde{\mu}_1, \tilde{\nu}_1$ | −                                                                                                                                                                     |
| −2  | $\mu_1, \nu_1, \tilde{\nu}_0$                              | $\mathcal{S}_1^{(0)}$                                                                                                                                                 |
| 0   | $\mu_0, \nu_0$                                             | $\mathcal{S}_0^{(0)}, \mathcal{S}_2^{(0)}, \mathcal{S}_1^{(1)}, \tilde{\mathcal{S}}_1^{(0)}$                                                                          |
| +2  | −                                                          | $\mathcal{S}_0^{(1)}, \mathcal{S}_2^{(1)}, \mathcal{S}_1^{(2)}, \mathcal{S}_1^{(3)}, \tilde{\mathcal{S}}_1^{(1)}, \tilde{\mathcal{S}}_2^{(0)}, \tilde{\mathcal{S}}_1$ |
| +4  | −                                                          | $\mathcal{S}_0^{(2)}, \mathcal{S}_2^{(2)}, \mathcal{S}_0^{(3)}, \mathcal{S}_2^{(3)}, \tilde{\mathcal{S}}_2^{(1)}$                                                     |

The numerical values of the complex coefficients are given in these units by (the coefficient  $\tilde{\mu}_1$  remains undetermined so far):

| $n$ | $\mu_n$                    | $\nu_n$                             | $\tilde{\nu}_n$                          | $\tilde{\mu}_n$ |
|-----|----------------------------|-------------------------------------|------------------------------------------|-----------------|
| 0   | $+3.8(4) - i0.570(2)$      | $-4.7(3) - i2.37(10) \cdot 10^{-2}$ | $-2.04(1.2) + i4.8(5) \cdot 10^{-4}$     | −               |
| 1   | $-676.1(4.0) + i7.27(2)$   | $+26.7(2.8) + i0.30(1)$             | $+433.2(12.2) - i6.0(1.3) \cdot 10^{-4}$ | n.d.            |
| 2   | $+559.7(18.5) - i16.80(5)$ | $-46.0(14.2) - i0.74(3)$            | −                                        | −               |
| 3   | $-1072.6(13.6) + i7.57(2)$ | $+123.9(12.6) - i0.28(1)$           | −                                        | −               |

The ancillary files provide the numerical tables for the set of fundamental solutions as functions of  $s$  according to the following correspondence:

$$\begin{aligned} \text{S\_n.dat} & \quad \mathcal{S}_I^{(n)}(s) & \quad I = 0, 1, 2, n = 0, 1, 2, 3 \\ \text{St\_n.dat} & \quad \tilde{\mathcal{S}}_I^{(n)}(s) & \quad I = 1, 2, n = 0, 1 \\ \text{St1.dat} & \quad \tilde{\mathcal{S}}_1(s) \end{aligned}$$

Each of the files S\_n.dat displays seven columns. The first column gives the value of  $s$  in  $\text{GeV}^2$ . The remaining six columns give successively the corresponding values of the functions  $\text{Re } \mathcal{S}_0^{(n)}(s)$ ,  $\text{Im } \mathcal{S}_0^{(n)}(s)$ ,  $\text{Re } \mathcal{S}_1^{(n)}(s)$ ,  $\text{Im } \mathcal{S}_1^{(n)}(s)$ ,  $\text{Re } \mathcal{S}_2^{(n)}(s)$ ,

\* veronique.bernard@ijclab.in2p3.fr

† sebastien.descotes-genon@ijclab.in2p3.fr

‡ knecht@cpt.univ-mrs.fr

§ bachir.moussallam@ijclab.in2p3.fr

$\text{Im } \mathcal{S}_2^{(n)}(s)$ , in units of  $\text{GeV}^N$ , with  $N$  as specified above. The two files **St\_n.dat** display five columns each, the first one giving the value of  $s$  in  $\text{GeV}^2$ . The four remaining columns give successively the values of the functions  $\text{Re } \tilde{\mathcal{S}}_1^{(n)}(s)$ ,  $\text{Im } \tilde{\mathcal{S}}_1^{(n)}(s)$ ,  $\text{Re } \tilde{\mathcal{S}}_2^{(n)}(s)$ ,  $\text{Im } \tilde{\mathcal{S}}_2^{(n)}(s)$  in the appropriate units of  $\text{GeV}^N$ . Finally, the last file, **St1.dat**, contains three columns displaying successively the values of  $s$ ,  $\text{Re } \tilde{\mathcal{S}}_1(s)$  and  $\text{Im } \tilde{\mathcal{S}}_1(s)$ , all in units of  $\text{GeV}^2$ . The range of values of  $s$  that is covered in the files is  $-2 \text{ GeV}^2 \leq s \leq 10 \text{ GeV}^2$ .

Also provided are the numerical values of the  $S$  and  $P$ -wave  $\pi\pi$  phase-shifts  $\delta_0(s)$ ,  $\delta_1(s)$ ,  $\delta_2(s)$  from which the solutions of the KT equations have been computed. They are given in the three files: **phase00+omnes00.dat**, **phase11+omnes11.dat** and **phase02+omnes02.dat**. In each of these files the numbers in the first column correspond to  $s$  (in  $\text{GeV}^2$ ), those in the second and third column to the phase-shift (in radians) and to the absolute value of the Omnès function (dimensionless).
